# Supplementary material for: Dynamic magnetism in the disordered hexagonal double perovskite BaTi$_{1/2}$Mn$_{1/2}$O$_{3}$
Source: arXiv:1802.09950 source file (2019-02-11)
Supplement: Supplementary file 1 [file 2018Cantarinoetall_spinliquidBTM0_suppv04.pdf]

# Supplemental material for: Dynamic magnetism in the Disordered Hexagonal Double Perovskite $BaTi_{1/2}Mn_{1/2}O_3$

M.R. Cantarino[1], R.P. Amaral[2], R.S. Freitas[1], J.C.R. Araújo[2], R. Lora-Serrano[2], H. Luetkens[3], C. Baines[3], S. Bräuninger[4], V. Grinenko[4], R. Sarkar[4], H.H. Klauss[4], E. C. Andrade[5], F. A. Garcia[1]
[1]*IFUSP, Univ. de São Paulo, 05508-090, São Paulo-SP, Brazil*
[2]*Univ. Fed. de Uberlândia, Instituto de Física, 38400-902, Uberlândia-MG, Brazil*
[3]*Laboratory for Muon Spin Spectroscopy, PSI, CH-5232 Villigen PSI, Switzerland*
[4]*Institute for Solid State and Material Physics, TU Dresden, D-01069 Dresden, Germany and*
[5]*Instituto de Física de São Carlos, Universidade de São Paulo, C.P. 369, São Carlos, SP, 13560-970, Brazil*

Here we present in detail some aspects of the data treatment, complementary data and some explanatory notes to give support to our discussion in the main text. In turn, we give details about 1) Resonant X-Ray Diffraction experiments and analysis; 2) analysis of $\chi(T)$ (that can be found on our previous paper Ref. [1]); 3) heat capacity analysis, with *a*) Fittings of $C_{\text{mag}}$; *b*) phonon subtraction and *c*) analysis of the Schottky anomalies; 4) $\mu SR$ analysis with *a*) dynamic spin susceptibility analysis (to determine the spin relaxation rates discussed in the main text) and *b*) investigation of the muon local environment.

## I. RESONANT X-RAY DIFFRACTION

The X-Ray diffraction experiments were carried out for incident photon energies 6500 eV, 6535 eV, 6564 eV and 12000 eV. The selected energies correspond, respectively, to below, slightly below, slightly above and greatly above the Mn absorption K-edge of 6539 eV. The FullProf software package [2] was adopted for the data refinement, during which several structural models were tested. The goal of this investigation is to probe the occupation of the transition metal sites $M(1)$, $M(2)$ and $M(3)$. Therefore, for each tested model we adopt a distinct, and fixed, occupation for the transition metal sites. The proposed model, as discussed in the main text and in Refs. [1, 3, 4], states that the $M(1)$ sites are occupied exclusively by Mn atoms, $M(3)$ exclusively by Ti atoms and $M(2)$ have mixed occupancy.

The statistics of the refinements were compared. Given the quality of the data and the difficulty to refine resonant X-ray diffraction, we choose to fix the occupancies using different models, as shown in table I, where Model 1 refers to the proposed model as mentioned above. It is supposed that the $M(1)$ site is always fully filled by Mn. This is based on the fact that the average bond length between $M(1)$ and O(1) corresponds closely to the value expected for Mn - O bonds.

Models including small changes in the proposed occupancy could still give a good description of the data. However, the statistics of the current model (model 1) was systematically better, specially in the cases of the near resonance data. When large deviations from the proposed model were tested, it incurred in much worse statistics. In Fig.S1($a$)-($d$) we show the refinement results for our model. Some peaks in the low angle region are not represented by the refinement because they correspond to peak residuals from the background subtraction and peaks originated from starch, that was used to dilute the sample in order to avoid the detector saturation.

The refinement results are also presented in tables II-V. During the refinement, we targeted the minimization of $\chi^2$, that was adopted as our statistical factor for judging the quality of the refinements. Also, it should be noted that for the resonance region, the Debye-Waller coefficient and the oxygen positions were not refined.

| Model1 | | |
|---|---|---|
| Site | Mn | Ti |
| M(1) | 100% | 0% |
| M(2) | 50% | 50% |
| M(3) | 0% | 100% |

| Model2 | | |
|---|---|---|
| Site | Mn | Ti |
| M(1) | 100% | 0% |
| M(2) | 45% | 55% |
| M(3) | 10% | 90% |

| Model3 | | |
|---|---|---|
| Site | Mn | Ti |
| M(1) | 100% | 0% |
| M(2) | 40% | 60% |
| M(3) | 20% | 80% |

Table I. Different models used to refine the resonant X-ray diffraction data and its relative atom occupancy in the sites$M(2)$ and $M(3)$.

M1: 6500 eV

| Atom | Site | Occupancy | x | y | z | $B_{iso}$ (Å$^2$) |
|---|---|---|---|---|---|---|
| Ba(1) | 6c | 1.0 | 0 | 0 | 0.286 (1) | 0.05 |
| Ba(2) | 6c | 1.0 | 0 | 0 | 0.129 (1) | 0.05 |
| M(1) Mn | 3b | 1.0 | 0 | 0 | 0.5 | 0.05 |
| M(2) Mn/Ti | 6c | 0.5/0.5 | 0 | 0 | 0.403 (2) | 0.05 |
| M(3) Ti | 3a | 1.0 | 0 | 0 | 0 | 0.05 |
| O(1) | 18f | 1.0 | 0.151 | 0.849 | 0.457 | 0.05 |
| O(2) | 18f | 1.0 | 0.167 | 0.833 | 0.627 | 0.05 |

$a = b = 5.690(5)$Å, $c = 27.90(4)$ Å, $\chi^2 = 4.55$

Table II. Refinements results for X-ray incident energy of 6500 eV and using the model 1 for the occupancy.

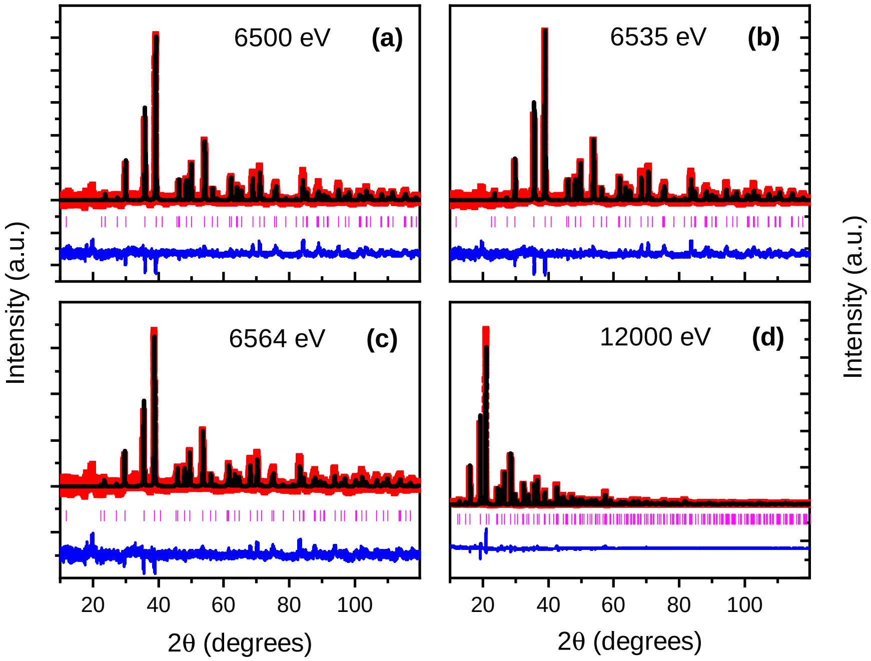


Figure 1. Refinements of X-ray diffraction for incident photon energy as indicated (the Mn K-edge sits at 6539 eV). The occupancies were fixed according to Model 1 in table I.

M1: 6535 eV

| Atom | Site | Occupancy | x | y | z | Biso (Å²) |
|---|---|---|---|---|---|---|
| Ba(1) | 6c | 1.0 | 0 | 0 | 0.286 (1) | 0.05 |
| Ba(2) | 6c | 1.0 | 0 | 0 | 0.129 (1) | 0.05 |
| M(1) Mn | 3b | 1.0 | 0 | 0 | 0.5 | 0.05 |
| M(2) Mn/Ti | 6c | 0.5/0.5 | 0 | 0 | 0.402 (2) | 0.05 |
| M(3) Ti | 3a | 1.0 | 0 | 0 | 0 | 0.05 |
| O(1) | 18f | 1.0 | 0.151 | 0.849 | 0.457 | 0.05 |
| O(2) | 18f | 1.0 | 0.167 | 0.833 | 0.627 | 0.05 |

"$a = b = 5.688(5)$ Å, $c = 27.89(4)$ Å, $\chi^2 = 4.51$"

Table III. Refinements results for X-ray incident energy of 6535 eV and using the model 1 for the occupancy.

M1: 6564 eV

| Atom | Site | Occupancy | x | y | z | Biso (Å²) |
|---|---|---|---|---|---|---|
| Ba(1) | 6c | 1.0 | 0 | 0 | 0.286 (1) | 0.05 |
| Ba(2) | 6c | 1.0 | 0 | 0 | 0.129 (1) | 0.05 |
| M(1) Mn | 3b | 1.0 | 0 | 0 | 0.5 | 0.05 |
| M(2) Mn/Ti | 6c | 0.5/0.5 | 0 | 0 | 0.402 (3) | 0.05 |
| M(3) Ti | 3a | 1.0 | 0 | 0 | 0 | 0.05 |
| O(1) | 18f | 1.0 | 0.151 | 0.849 | 0.457 | 0.05 |
| O(2) | 18f | 1.0 | 0.167 | 0.833 | 0.627 | 0.05 |

"$a = b = 5.687(6)$ Å, $c = 27.89(4)$ Å, $\chi^2 = 2.97$"

Table IV. Refinements results for X-ray incident energy of 6564 eV and using the model 1 for the occupancy.

M1: 12000 eV

| Atom | Site | Occupancy | x | y | z | Biso (Å²) |
|---|---|---|---|---|---|---|
| Ba(1) | 6c | 1.0 | 0 | 0 | 0.2856 (3) | 0.54 (2) |
| Ba(2) | 6c | 1.0 | 0 | 0 | 0.1286 (3) | 0.21 (2) |
| M(1) Mn | 3b | 1.0 | 0 | 0 | 0.5 | 0.16 (4) |
| M(2) Mn/Ti | 6c | 0.5/0.5 | 0 | 0 | 0.4071 (8) | 0.35 (4) |
| M(3) Ti | 3a | 1.0 | 0 | 0 | 0 | 0.42 (4) |
| O(1) | 18f | 1.0 | 0.148 (4) | 0.852 (4) | 0.457 (2) | 0.11 (7) |
| O(2) | 18f | 1.0 | 0.154 (6) | 0.846 (6) | 0.629 (2) | 0.17 (9) |

"$a = b = 5.6934(3)$ Å, $c = 27.922(2)$ Å, $\chi^2 = 5.18$"

Table V. Refinements results for X-ray incident energy of 12 keV and using the model 1 for the occupancy.

## II. SUSCEPTIBILITY

The detailed analysis of the high temperature susceptibility ($\chi(T)$) was the subject of a previous paper by some of the authors [1]. Here, we give a fast account of this previous discussion in order to set the context. The magnetic properties of the paramagnetic state is rooted in the structural model. In Reference to Fig.1(a) in the main text, the $BaTi_{1/2}Mn_{1/2}O_3$ unit cell contains 3 $M(1)$ and $M(3)$ sites and 6 $M(2)$ sites. All sites occupied by Mn atoms are inside the structural trimers ($M(1)$ and $M(2)$ sites). The $M(1)$ and $M(2)$ sites are inside face sharing oxygen octahedra, giving rise to a large multiplicity of exchange paths. As a consequence, one may expect the exchange coupling between the Mn cations to be large. We name $J_1$ the first neighbor super-exchange constant and $J_2$ the second neighbor super-super-exchange (indicated Fig.1(b) of the main text). These are effective constants taking into account all multiplicity of the exchange paths.

Considering the disordered occupancy, there are 4 possible configurations for the occupancy of the structural trimers, given the 2 possible filling of both $M(2)$ sites in the structural trimers. 3 Mn cations, 2 Mn cations plus 1 Ti cation (in two different orders) and 1 Mn cation plus 2 Ti cations. Each of these configurations will, respectively, give the following contributions to $\chi(T)$: magnetic trimers ($\chi(T)_{\text{trim}}$), magnetic dimers $\chi(T)_{\text{dim}}$and orphan spins $\chi(T)_{\text{orp}}$.

Concerning the fraction of each of these magnetic units, given the 4 possible fillings above that amount for a total of 8 Mn and 4 Ti, we can therefore conclude that 3/8 of the Mn atoms will form trimers, 4/8 will form dimers and 1/8 will be orphans, resulting in 1/8 mols of magnetic trimers and orphan spins per mol of Mn and 2/8mols of magnetic dimers per mol of Mn.

The dimer contribution, can be deduced from the following Hamiltonian:

$$\mathcal{H}_{\text{dimer}} = J_1 \boldsymbol{S}_1.\boldsymbol{S}_2 \tag{1}$$

The trimer contribution, can be deduced from the following Hamiltonian:

$$\mathcal{H}_{\text{trim}} = J_1 \boldsymbol{S}_1.\boldsymbol{S}_2 + J_1 \boldsymbol{S}_2.\boldsymbol{S}_3 + J_2 \boldsymbol{S}_1.\boldsymbol{S}_3 \tag{2}$$

As for the orphan spins, its contribution are modeled by a Curie-Weiss type susceptibility:

$$\chi(T) = \frac{C_{\text{orp}}}{T - \theta_{\text{orp}}} + \chi_0 \tag{3}$$

The obtained parameters are: $J_1 = 176(7)$ K, $J_2 = 0.59 J_1$, $\theta_{\text{orp}} = -6.8(2)$ K and $C_{\text{orp}} = 0.13(1)$ emu.K/Oe.mol (f.u.). The numbers are slightly different than previously [1] mostly for three reasons: (1) the restricted temperature interval ($T > 5.5$ K); (2) new, and improved, sample batch. We call attention that $C_{\text{orp}} = 0.13(1)$ emu.K/Oe.mol (f.u.) must be compared with $C \approx 0.12$ emu.K/Oe.mol (f.u.) expected for 1/16 mols of Mn $S = 3/2$ spins per formula unit of $BaTi_{1/2}Mn_{1/2}O_3$ (half mol of Mn), which is a very good agreement.

For $J_1 = 176(7)$ K, $J_2 = 0.59 J_1$, the ground state of a trimer is an effective $S = 1/2$ spin with the first excited state lying $\approx 38$ K above the ground state. Therefore, the remaining magnetic degrees of freedom at low-$T$ are effective $S = 1/2$ spins due to all trimers and the $S = 3/2$ spins due to orphans. As discussed in the main text, the data in Fig.2$c$ supports the existence of correlated spins at low$-T$, that we now identify as a state formed by $S = 1/2$ and

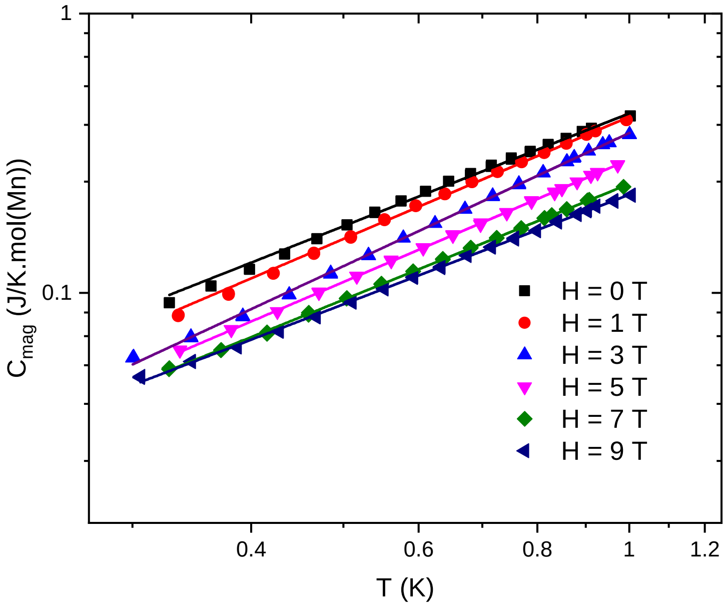


Figure 2. Fittings of the low $T$ region ($0.2 \leq T \leq 1.0$ K) of $C_{\mathrm{mag}}(T)$ data to the expression: $C_{\mathrm{mag}}(T) = \gamma(H)T^{\alpha(H)}$ for different values of $H$

$S = 3/2$ spins. To estimate the interactions among the remaining magnetic degrees of freedom, we resort to a mean field approximation [5]considering coupled $S = 3/2$ and $S = 1/2$ spins.

The resulting effective energy scale is $\theta_{\mathrm{eff}} = -7.5(1)$ K, and we can conclude that this correlated state of orphans and trimers is also highly frustrated (since no phase transition is observed down to 0.1 K, the frustration parameter $f$ is at least $f \gtrsim 75$). The resulting Curie constant is $C_{\mathrm{eff}} = 0.19(1)$ emu.K/Oe.mol (f.u.) which compares well with the expected $\approx 0.14$ emu.K/Oe.mol (f.u.), and supports our scenario.

## III. HEAT CAPACITY

### A. Low-$T$ fitting of $C_{\mathrm{mag}}$

The behavior of $C_{\mathrm{mag}}$ at low$-T$ is key to characterize our proposed spin liquid phase. In the main text (Fig. 2), we reported $\alpha(H)$ and $\gamma(H)$ parameters obtained by fitting $C_{\mathrm{mag}}$ to the expression:

$$C_{\mathrm{mag}}(T) = \gamma(H)T^{\alpha(H)}$$

the fitting considered the following data range $0.25 \leq T \leq 1.2$ K. We adopt that in this $T$-interval the phonon contribution to the heat capacity is negligible (see discussion below). Furthermore, we start our fitting at $T = 0.25$ K since the contribution from the Mn nuclear heat capacity can be discarded as well. In Fig.S2 we show the fitting results in detail. As usual, to calculate $\Delta S$ in the main text, the $H = 0$ data was extrapolated to $T = 0$ employing the fitting results here discussed.

### B. Subtraction of the phonon contribution

Our main objective is to extract the magnetic heat capacity from the heat capacity data $C_p$ in order to: 1) characterize the excitation of the proposed spin liquid phase in the low temperature region (to be understood as $0.2 \leq T \leq 1.2$ K) and 2) to evaluate the total entropy recovered up to $T = 10$ K. The total heat capacity includes two contributions:

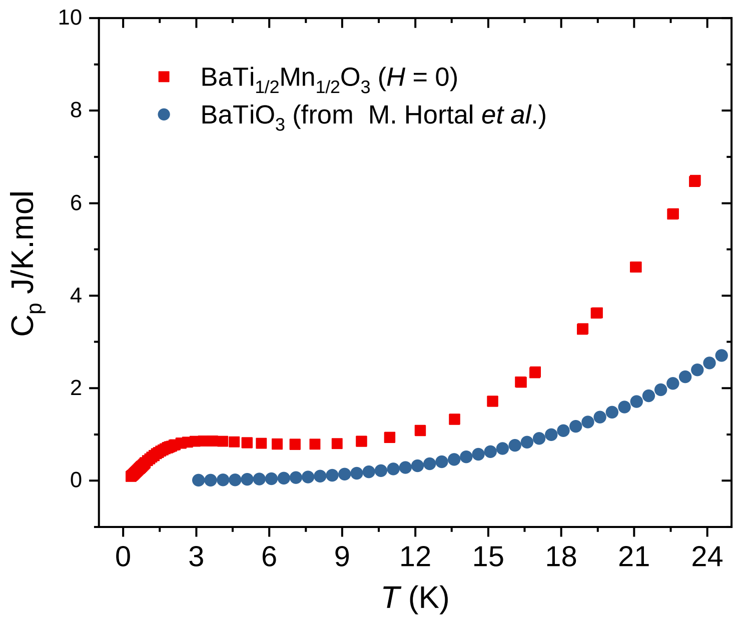


Figure 3. $BaTi_{1/2}Mn_{1/2}O_3$ heat capacity data ($H = 0$) compared with the $BaTiO_3$ heat capacity (from Ref. [6]) . At $T = 3$ K, the $BaTiO_3$ $C_p$ is 3 orders of magnitude smaller than the $C_p$ of our sample. .

$$C_p = C_{\mathrm{lattice}} + C_{\mathrm{mag}}$$

In the absence of a suitable non magnetic reference compound, we will proceed as follows: $i$) as already discussed, at the low temperature region, the phonon contribution is negligible. ; ii) for $T$ up to $\approx 10$ K, however, the phonon contribution cannot be completely ignored and we adopt the $BaTiO_3$ heat capacity as a non-magnetic reference. In Fig. S3, $C_p$ of our sample ($H = 0$) is compared with $C_p$ of the cubic perovskite $BaTiO_3$ [6].

It must be appreciated that while it is robust to ignore the phonon contribution to $C_p$ for $T$ up to 1.2 K, adopting the $BaTiO_3$ heat capacity as a reference is only an approximation. However, it does not change significantly the scenario being proposed. For instance, the total entropy $\Delta S$ recovered when no subtraction is employed is 2.04 J/K.mol(Mn), which is to be compared with 1.97 J/K.mol(Mn) that is obtained after the subtraction.

In Fig.3($a$) of the main text, the $C_{\mathrm{mag}}$ data was obtained by subtracting the $BaTiO_3$ $C_p$ up to $T = 8$ K. Again, we emphasize that no parameter being discussed in the paper, except the value of $\Delta S$, depends upon this subtraction.

In Fig.4 we display the full low$-T$ heat capacity including the upturn that we ascribe to the Mn nuclear heat capacity as discussed in the main text.

### C. Schottky anomaly due to trimers

As discussed in the main text, the presence of uncorrelated magnetic trimers would imply the appearance of sizable Schottky anomalies in the field dependent measurements of the magnetic heat capacity $C_{\mathrm{mag}}$. Here we show the details of this discussion. We will also present the results for the dimer contribution, showing that it can be ignored in the low-$T$ region.

Adopting the experimentally determined $J_1$ and $J_2$ values and Hamiltonians in Eqs. (2) and (1) (including an extra Zeeman term), the energy levels of the magnetic trimer and dimer states can be calculated. The results are then applied to calculate the contribution of the magnetic trimers to $C_{\mathrm{mag}}$:

$$C_{\mathrm{mag}} = \frac{\partial}{\partial T} \sum_n E_n \exp(-E_n/k_B T)$$

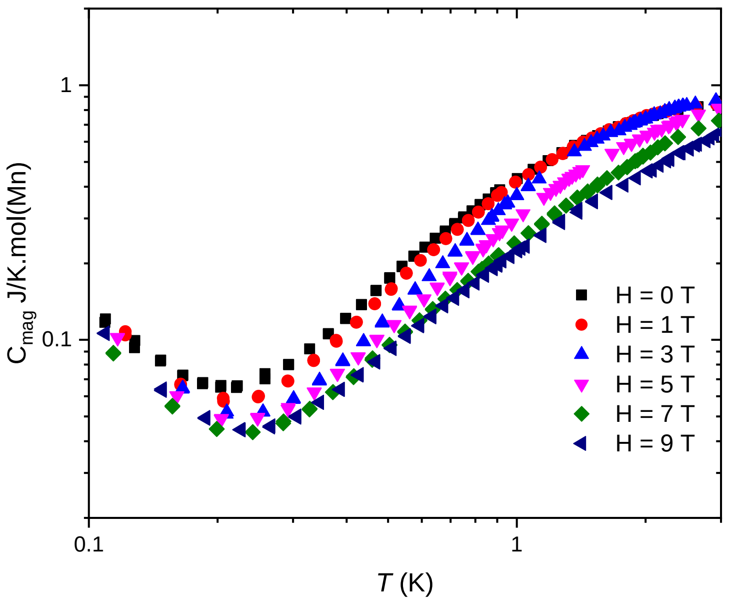


Figure 4. $C_{\rm mag}(T)$ in the low $T$ region for distinct values of $H$. For $T < 0.1$ K, $C_{\rm mag}$ display the dominant contribution from the Mn Nuclear degrees of freedom.

Results are presented in Fig. S5(a)-(b). As expected, dimers do not present the anomaly for its ground state is a singlet. Furthermore, the dimer contribution to the total entropy in this temperature range is negligible since $C_{\rm dimer} \approx 0$ (and the entropy recovering associated do the dimer formation takes place at higher temperature). The trimer, however, would present a sizable contribution that can be compared with experimental data. This comparison is presented in Fig. S5(c) for $H = 1$T and $H = 9$ T. At this selected fields, it is clear that the sole contribution of the trimer would be larger than $C_{\rm mag}$. In conclusion, it is suggested once again that the magnetic trimers are part of the proposed correlated state.

## IV. $\mu$SR

### A. Dynamic spin susceptibility

Now we present details of a brief quantitative analysis of the $\mu$SR experimental results. Our aim is to estimate the spin fluctuation rate for temperatures above and below the crossover. Here, we closely follow the discussion of Refs. [7, 8]. The spin fluctuation rate $\nu$ for $T > 10$ K can be estimated as:

$$\nu_{T>10\text{ K}} = zJS/h$$

where $z$ is the coordination number of the magnetic lattice, $J$ is the exchange constant, $S$ is the spin of the magnetic specimen and $h$ the Planck constant . In reference to Fig.1(c) of the main text, $z = 6$. In a mean field approximation, $J$ can be calculated from $\theta_{\rm orp} = -7.3$ K as:

$$\theta_{\rm orp} = z\frac{JS(S+1)}{3}$$

The results are $J \approx 0.97$ K and $\nu_{T>10\text{ K}} = 7.4(1) \times 10^{10}$ Hz as written in the main text. Another parameter of interest is the field distribution width $\Delta$. In general:

$$\lambda(H) = \frac{2\nu\Delta^2}{\nu^2 + (\mu_0 H^2 \gamma_\mu)^2}$$

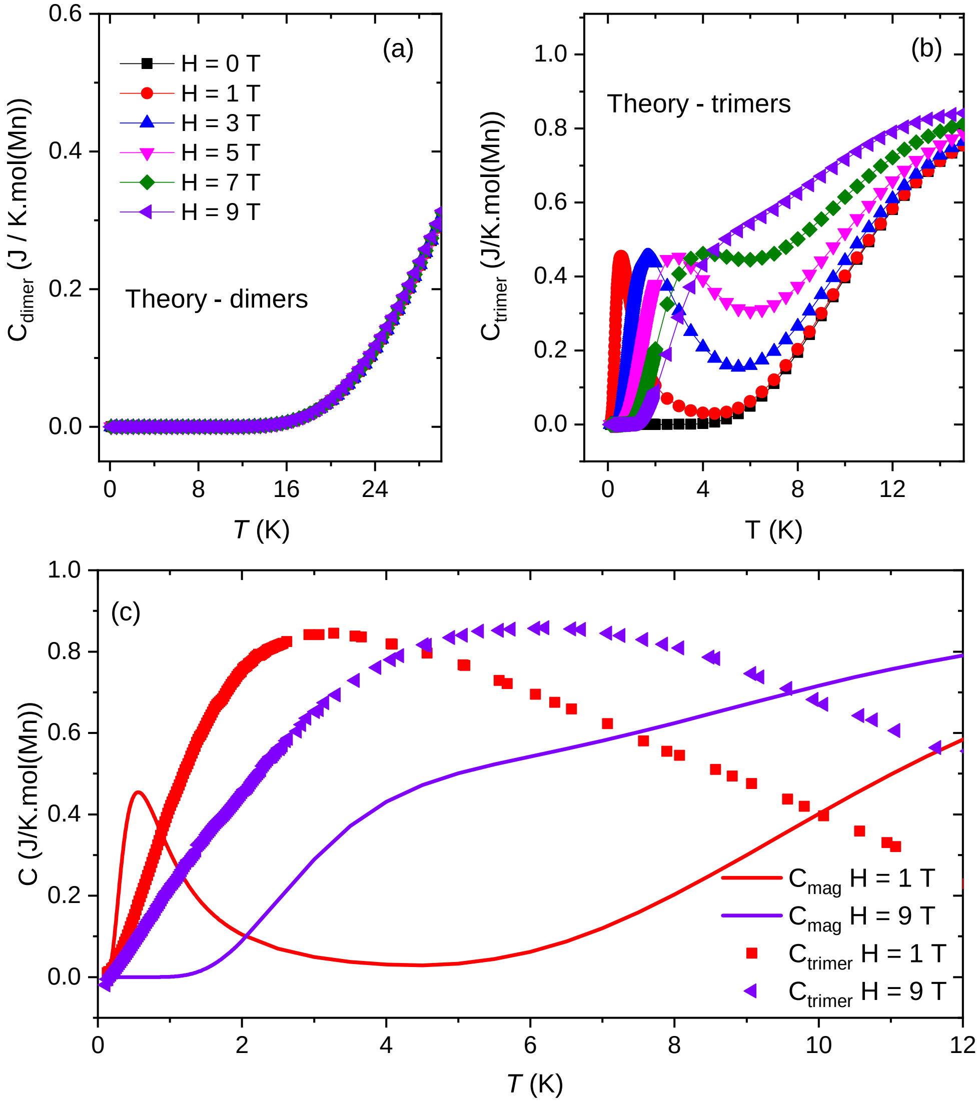


Figure 5. Theoretical analysis of the magnetic heat capacity due to dimers and trimers and comparison to experimental data. (a)-(b) Dimer and trimer contribution to the magnetic heat capacity as a function of $H$ (energy levels calculated from the Hamiltonians given by Eqs. 2 1, experimentally determined $J_1$ and $J_2$ ). Both contribution are negligible for $H = 0$. Furthermore, up to $T = 15$ K the dimer contribution can always be neglected. (c) Comparison between the calculated trimer Schottky anomaly and experimental data.

where $\lambda$is the nearly $T-$independent relaxation rate for $T > 10$ K ($\lambda \approx 0.07\ \mu s^{-1}$, see Fig. 4(c) of the main text) , $\mu_0 H$ is the applied magnetic field (which is 0) and $\gamma_\mu$ is the muon gyromagnetic factor (135.5 MHz/T). We obtain $\Delta = 5.09 \times 10^7$ Hz.

The above equations are not appropriate for the low$-T$ region. Indeed, it is expected that at low$-T$, the spin dynamic autocorrelation function $S(t)$ will be $S(t) \propto (\tau/t)^x \exp(-\nu t)$ with $x \neq 0$, since the system is not a simple paramagnet. In this case, the formula for $\lambda(H)$ assumes the following form [8]:

$$\lambda(H) = 2\Delta^2 \tau^x \int_0^\infty t^{-x} \exp(-\nu_{T<1.5\ \mathrm{K}} t) \cos(2\pi\mu_0\gamma_\mu H t) dt$$

where$\tau$ is early time cutoff, $\Delta$ is the new field distribution width (for the low$-T$ region) , $x$ is a critical exponent and $1/\nu$ is the late time cutoff (spin fluctuation rate) . The experimental values for $\lambda(H)$ are extracted from the LF

experiments. The obtained parameters are $x = 0.64(3)$ and $\nu_{T<1.5\text{ K}} = 3.7(6) \times 10^6$ Hz. This is a decrease of about 4 orders of magnitude when compared with $\nu_{T>10\text{ K}}$. Fig S6 show the data and the fitting. This result should be taken with care in view of the small amount of data points for distinct field values in the LF experiments. Nevertheless, it suggests long-time spin correlations at low$-T$ in our system.

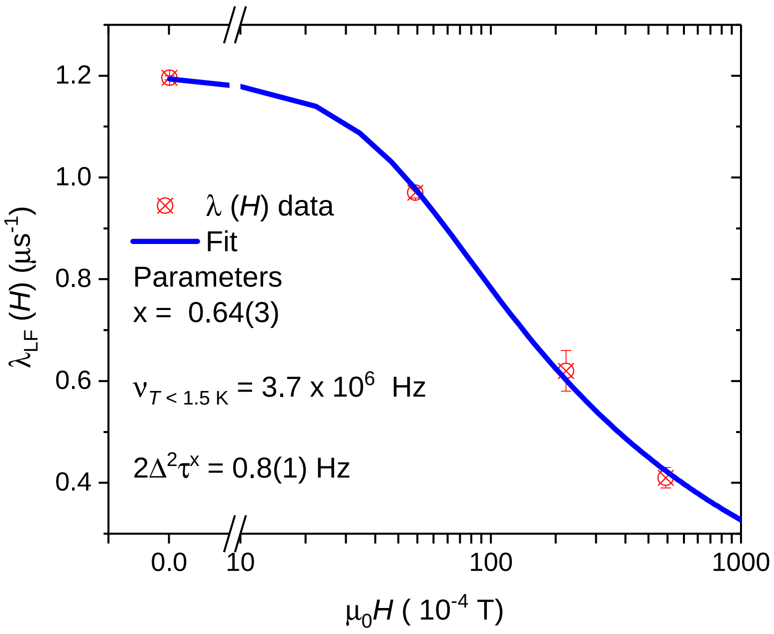


Figure 6. Relaxation rate as a function of $H$ (crossed circles) and the fitting of $\lambda(H)$ as discussed in the text.

### B. Muon local environment

We performed DFT calculations of the unperturbed unit cell of the electrostatic potential of $BaTi_{0.5}Mn_{0.5}O_3$ to estimate roughly the possible muon site. DFT calculations were performed using the all-electron full-potential linearized augmented-plane wave (FP-LAPW) code Elk 4.3.6 which includes the Spacegroup package using Broyden mixing [9] and the Perdew-Burke-Ernzerhof-GGA (Generalized gradient approximation) functional [10]. The unit cell of $BaTi_{0.5}Mn_{0.5}O_3$ contains 88 atoms as presented in this paper and elsewhere [1, 3, 4]. This assumes the hexagonal space group $R\bar{3}m$:H (No.1) in the Herrman-Mauguin notation. The crystal system, the Bravais lattice is trigonal of $R\bar{3}m$:H. The symmetry is $D_{3d}$ in Schönflies notation. The second representation, $R\bar{3}m$:R (No.2), takes a rhombohedral axis and contains 27 atoms. Therefore, we have chosen the space group $R\bar{3}m$:R (No.2) for the DFT calculation to reduce the calculation time significantly. Table VI shows the calculated values of $R\bar{3}m$:R (No.2) started from the values of Ref. [1]. The adopted unit cell is rhombohedral with:

$$\angle(a, b) = \angle(a, c) = \angle(b, c) = 33.5189^\circ. \tag{4}$$

The adopted length of the unit cell is taken to be 18.64794971 $a_0$ where $a_0$ is the atomic Bohr radius $a_0$.

Figure 7 shows this unit cell with two different values of the electrostatic potential represented by the yellow isosurfaces . The diagonal line of the unit cell of $R\bar{3}m$:R corresponds to the c-axis of $R\bar{3}m$:H. The disordered ions $Mn^{4+}$ and $Ti^{4+}$ are close to the sharp edges. The disorder of $Mn^{4+}$ and $Ti^{4+}$ is handled in the following way: the primitive $R\bar{3}m$:R-cell contains two transition metal elements and one is chosen to be Mn and the second one Ti. Statistically, this is assumed to be the most represented case. The muon carries a positive charge and should be located close to $O^{2-}$. The electrostatic energy minimum below $\varphi$ of the undistorted unit cell is located inside the yellow structures of Fig.7. The lowest energy minima are insight the flower structures of figure 7 (b). The isosurface structures are slightly asymmetric because of the mentioned assumption of one Ti and one Mn of the 6$c$ site leading to an asymmetric unit cell. Therefore it can be that the muon site closer to a disordered Mn is slightly preferred.

| Element | Site | x | y | z |
|---|---|---|---|---|
| Ba(1) | 6c | 0.2856(2) | 0.2856(2) | 0.2856(2) |
| Ba(2) | 6c | 0.1290(2) | 0.1290(2) | 0.1290(2) |
| M(1)(Mn) | 3b | 0.5 | 0.5 | 0.5 |
| M(2)(Ti/Mn) | 6c | 0.4091(2) | 0.4091(2) | 0.4091(2) |
| M(3)(Ti) | 3a | 0 | 0 | 0 |
| O(1) | 18f | 0.60786(2) | 1.15396(2) | -0.39214(1) |
| O(2) | 18f | 0.7943(2) | 1.2924(2) | -0.62057(1) |

Table VI. Structure parameters of $BaTi_{0.5}Mn_{0.5}O_3$ of the space group $R\bar{3}m$:R at room temperature. The calculation is based on the values from Ref.[1]. The space group is $R\bar{3}m$:R (spacegroup number 166) with $a = b = c = 9.86807(9)$ Å. The $M$(1-3) sites are the transition metal sites.

(a)

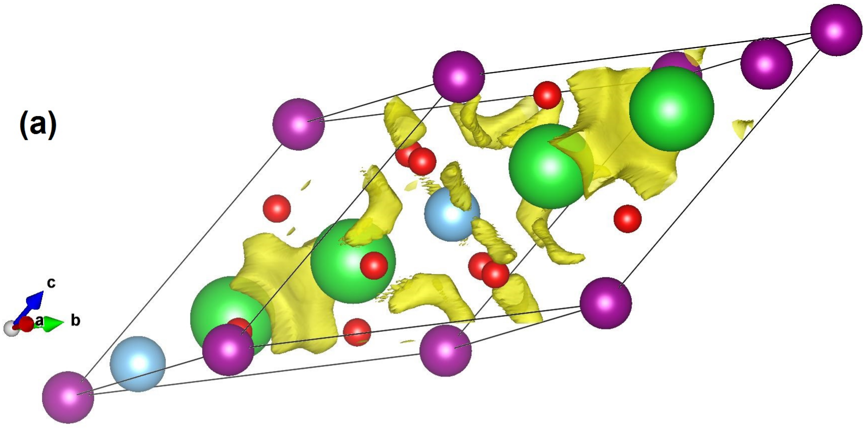


(b)

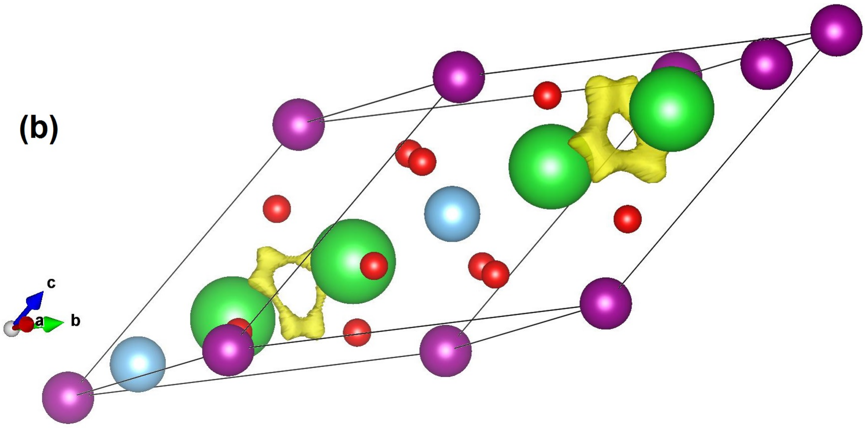


Figure 7. The unit cell of $BaTi_{0.5}Mn_{0.5}O_3$ of the space group $R\bar{3}m$:R is visualized by the atomic radii. Barium atoms are shown in green, Oxygen in red, Titanium in blue and Manganese in purple. The yellow isosurface represents the electrostatic potential $\varphi$ of ($a$) -0.45 $\frac{E_h}{e}$ and ($b$)-0.468 $\frac{E_h}{e}$.($a$) Two flower-like structures between Ba with holes and banana-like structures are observed in the middle of the unit cell. ($b$) The two flower structures are robust for decreasing electrostatic energy.

However, this result proposes that the muon is located close to Oxygen close to the Barium plane ignoring a possible muon-induced local lattice displacement.

[1] F. A. Garcia, U. F. Kaneko, E. Granado, J. Sichelschmidt, M. Hölzel, J. G. S. Duque, C. A. J. Nunes, R. P. Amaral, P. Marques-Ferreira, and R. Lora-Serrano, Physical Review B **91**, 224416 (2015).

[2] J. Rodríguez-Carvajal, Physica B: Condensed Matter **192**, 55 (1993).
[3] G. M. Keith, C. A. Kirk, K. Sarma, N. M. Alford, E. J. Cussen, M. J. Rosseinsky, and D. C. Sinclair, Chemistry of Materials **16**, 2007 (2004).
[4] L. Miranda, A. Feteira, D. C. Sinclair, K. Boulahya, M. Hernando, J. Ramirez, A. Varela, J. M. Gonzalez-Calbet, and M. Parras, Chemistry of Materials **21**, 1731 (2009).
[5] M. T. Causa, M. Tovar, A. Caneiro, F. Prado, G. Ibanez, C. A. Ramos, A. Butera, B. Alascio, X. Obradors, S. Pinol, *et al.*, Physical Review B **58**, 3233 (1998).
[6] M. Hortal, S. Vieira, and R. Villar, Ferroelectrics **54**, 313 (1984).
[7] Y. J. Uemura, A. Keren, K. Kojima, L. P. Le, G. M. Luke, W. D. Wu, Y. Ajiro, T. Asano, Y. Kuriyama, M. Mekata, H. Kikuchi, and K. Kakurai, Physical Review Letters **73**, 3306 (1994).
[8] Y. Li, D. Adroja, P. K. Biswas, P. J. Baker, Q. Zhang, J. Liu, A. A. Tsirlin, P. Gegenwart, and Q. Zhang, Physical Review Letters **117**, 097201 (2016).
[9] G. P. Srivastava, Journal of Physics A: Mathematical and General **17**, L317 (1984).
[10] J. P. Perdew, K. Burke, and M. Ernzerhof, Physical Review Letters **77**, 3865 (1996).
